# Supplementary material for: SRHand: Super-Resolving Hand Images and 3D Shapes via View/Pose-aware Neural Image Representations and Explicit 3D Meshes
Source: arXiv:2509.21859 source file (2025-09-26)
Supplement: Supplementary file 1 [file supp.tex]

\PassOptionsToPackage{numbers, compress}{natbib}

\documentclass{article}

% if you need to pass options to natbib, use, e.g.:
% before loading neurips_2023

% ready for submission
\usepackage{Styles/neurips_2025_sup}

% to compile a preprint version, e.g., for submission to arXiv, add add the
% [preprint] option:
%     \usepackage[preprint]{neurips_2023}

% to compile a camera-ready version, add the [final] option, e.g.:
%     \usepackage[final]{neurips_2023}

% to avoid loading the natbib package, add option nonatbib:
%    \usepackage[nonatbib]{neurips_2023}

\usepackage[utf8]{inputenc} % allow utf-8 input
\usepackage[T1]{fontenc}    % use 8-bit T1 fonts
\usepackage{hyperref}       % hyperlinks
\usepackage{url}            % simple URL typesetting
\usepackage{booktabs}       % professional-quality tables
\usepackage{amsfonts}       % blackboard math symbols
\usepackage{nicefrac}       % compact symbols for 1/2, etc.
\usepackage{microtype}      % microtypography
\usepackage{xcolor}         % colors
\usepackage{svg}
\usepackage{pdfpages}
\usepackage{booktabs}
\usepackage{subcaption}
\setcitestyle{square}
\usepackage{multirow}
\usepackage{adjustbox}
\title{SRHand: Super-Resolving Hand Images and 3D Shapes via View/Pose-aware Neural Image Representations and Explicit 3D Meshes

- Supplementary Material - }

% \begin{document}

\maketitle

In this supplementary material, we provide more ablation experiments and discussions that are not included in the main paper due to the page limit.
% \twocolumn[{%
% \renewcommand\twocolumn[1][]{#1}%
% \begin{center}
% \centering
% \captionsetup{type=figure}
% \includegraphics[width=15cm]{ICCV2025-Author-Kit/fig/Illustrate.pdf}
% \caption{Taking a single image input, our method renders the personalized texture of two hands at novel views, poses, and light conditions.}
% \label{Teaser}
% \end{center}
% }]

\section{Details of Dataset}
We mainly use two datasets for experiments: InterHand2.6M \cite{sInterHand2.6M} and Goliath \cite{sgoliath}. Considering practical scenarios in the real world where the hand occupies less than 1\% from the full body captured image, we set the upscaling factor to $\times$ 16 in our main experiments. Furthermore, Sec. \ref{sec:arb} describes that our method achieves plausible results in any arbitrary upscaling factors.

\subsection{InterHand2.6M}
InterHand2.6M \cite{sInterHand2.6M} is constructed by capturing sequential frames from multi-view videos of single hands and two-hand interactions. For each frame, we crop the hand region and resize it to specific resolutions. To train GIIF, we use the \textit{'train'} split, with \textit{'Capture0' $\sim$ 'Capture22'} as the training dataset and the remaining captures (\textit{'Capture23' $\sim$ 'Capture26'}) as the validation dataset.

For 3D hand mesh reconstruction, we primarily use a single hand from the \textit{'test'} split, which differs from the GIIF training dataset, and incorporate identities from \textit{Capture0} and \textit{Capture1}. We use a sequence from \textit{ROM03\_RT\_No\_Occlusion}, following prior works. For the 3D reconstruction experiments, we sample 20 views with 20 frames. After training, we test on the \textit{'cam400262'} and \textit{'cam400263'} camera views with 398 frames. The results are reported as the mean value from both camera perspectives.

\subsection{Goliath}
Goliath \cite{sgoliath} provides high-resolution images of a single hand, including OLAT (one-light-at-a-time) captures and scanned meshes. Since our work does not strictly account for lighting conditions, we sample fully illuminated images. As the Goliath dataset does not provide ground truth MANO \cite{sMANO} parameters, we fit the MANO mesh to the UHM \cite{sUHM} template mesh using a joint loss for pose and translation parameters and Chamfer distance loss for the shape parameter. Once the MANO parameters are optimized, we use the 'test' split for 3D hand reconstruction of the subject 'AXE977'. Frames are sampled uniformly at fixed intervals, and evaluation is performed by skipping frames.

\section{Implementation Details}
\label{sec:rationale}
In this section, we provide more details on implementations of GIIF and prior work modifications.

\subsection{Geometric-aware Implicit Image Function}
Geometric-aware Implicit Image Function (GIIF) takes low-resolution images $I_{lr}$, and normal maps $N$ are extracted from the MANO \cite{sMANO} template mesh. $I_{lr}$ is encoded through the Residual Dense Network encoder \cite{sRDN}, and  $N$ is encoded through the stacked hourglass encoder \cite{sHG}. After extracting each embedded feature, we concatenate the latent features along the channel-wise dimension. Following LIIF \cite{sLIIF}, we employ cell decoding, local feature aggregation, and sample coordinates as queries in MLPs. After obtaining the predicted color for each query coordinate, we use adversarial learning with a discriminator. Our discriminator architecture is based on the UNet structure with spectral normalization.

We train GIIF for 20 epochs, after which we apply adversarial learning with our discriminator. The learning rate for GIIF is 0.0001, and for the discriminator, it is 0.001. Both are trained for 10 epochs.

\subsection{Geometric-aware LIIF}
Geometric-aware LIIF, denoted as LIIF$^*$ in this paper, geometric-aware LIIF is implemented similar to the GIIF. Compared to the GIIF, geometric-aware LIIF is not trained with adversarial learning. 

\subsection{Geometric-aware IDM }
We modify IDM to create a geometric-aware version, denoted as IDM$^*$ in this paper. IDM \cite{sIDM} is based on an encoder-decoder framework, where the decoder represents a continuous field and the encoder takes a normal map as a condition. Following conventional conditioning mechanisms, we incorporate a residual attention network and a style layer, enabling the encoder to output features that fuse both low-resolution (LR) image information and normal map details. The decoder then processes the concatenated feature representation to compute the target values based on query coordinates. This geometric-aware design enhances the model’s ability to preserve fine geometric details, resulting in sharper and more structured hand reconstructions.

\subsection{Universal Hand Model}
Since the Universal Hand Model (UHM) \cite{sUHM} is designed for single-view reconstruction, it is not adaptable for multi-view reconstruction. Thus, we train UHM on a single view and evaluate it with trained viewpoints, which benefits the testing conditions. In total, 400 frames are used, with 200 frames for training and the remaining frames for evaluation, ensuring a balanced and evenly distributed dataset. Although UHM has easier testing conditions, our method still achieves better results, as shown in Tab. 3 in the main paper.

\section{More Ablation Studies}
\subsection{Adaptive Fine-tuning}
We present the results of inconsistencies at each step to demonstrate the effectiveness of adaptive fine-tuning in Fig. \ref{abl_incon_time}. The SR module is fine-tuned every 50 steps, starting from the midpoint of the total epochs. We observe that inconsistencies tend to decrease while enhancing performance within the time step $t$ increases.
\begin{figure}[h]
  \centering
  \includegraphics[width=13.9cm]{fig/abl_incon_time.pdf}
  \caption{Qualitative results showing (a) inconsistencies in texture and (b) photometric performance variations over the time steps.}
  \label{abl_incon_time}
\end{figure}

We further validate the effectiveness of the adaptive fine-tuning process in the 3D reconstruction process at \ref{abl_training_loss}. Applying adaptive fine-tuning enables the 3D reconstruction model to converge more stably by addressing inconsistency issues.
\vspace{-0.2in}
\begin{figure}[h]
  \centering
  \includegraphics[width=9cm]{fig/training_plot.png}
  \caption{We plot 3D reconstruction training loss to show the effectiveness of adaptive fine-tuning. Mark "aft." stands for adaptive fine-tuning.}
  \label{abl_training_loss}
\end{figure}

\subsection{Effectiveness of Multi-View / Pose Consistency}
We present the results of the effectiveness of multi-view consistency and pose consistencies. Tab. \ref{abl_mv_pose} and Fig. \ref{abl_mv_pose_fig} show the quantitative and qualitative results, respectively. Each multi-view consistency and multi-pose consistency helps to increase consistencies between images; notably, applying both consistency loss shows better results.

\begin{table}[h]
\centering
\caption{Quantitative experiments of the effectiveness of multi-view consistency and multi-pose consistency.}
\label{abl_mv_pose}
\begin{adjustbox}{scale=0.88}
\begin{tabular}{@{}cc|cccc@{}}
\toprule
% \multicolumn{1}{l}{View Cons.} & \multicolumn{1}{l|}{Pose Cons.} & PSNR           & LPIPS           & SSIM             & P2P (mm)       \\ \midrule
%                                &                                 & 29.17          & 0.0404          & 0.9020           & 3.09           \\
% \checkmark                     &                                 & 27.08          & 0.0541          & 0.8882           & 3.23           \\
%                                & \checkmark                      & 28.05          & 0.0452          & 0.8975           & 3.04  \\
% \checkmark                     & \checkmark                      & \textbf{29.88} & \textbf{0.0362} & \textbf{0.9115}  & \textbf{2.16}           \\ \bottomrule
\multicolumn{1}{l}{View Cons.} & \multicolumn{1}{l|}{Pose Cons.} & PSNR (SR)     & PSNR           & LPIPS           & P2P (\textit{mm})       \\ \midrule
                               &                                 & 29.96         & 29.17          & 0.0404          & 3.09           \\
\checkmark                     &                                 & 29.99         & 27.08          & 0.0541          & 3.23           \\
                               & \checkmark                      & 30.01         & 28.05          & 0.0452          & 2.25  \\
\checkmark                     & \checkmark                      &\textbf{30.06} & \textbf{29.88} & \textbf{0.0362} & \textbf{2.16}           \\ \bottomrule
\end{tabular}
\end{adjustbox}
\end{table}

\begin{figure}[h]
  \centering
  \includegraphics[width=8cm]{fig/abl_mv_pose.pdf}
  \caption{Qualitative results of multi-view, multi-pose ablation study.}
  \label{abl_mv_pose_fig}
\end{figure}

\subsection{Statistical Significance}
We report the evaluation metrics averaged over 10 trials with different random seeds. The random seeds effect on the initial weight of MLP network in SRHand. As shown in Table~\ref{abl_stat}, we report the mean, p-value, and 1-sigma (standard deviation) error bars of 3D hand reconstruction from SR images experiment (InterHand2.6M \cite{sInterHand2.6M}) across the runs. To validate the reliability of the statistical reporting, we conducted a Shapiro-Wilk normality test for each metric. The results (p > 0.05 for all metrics) confirm that the distribution of errors can be considered approximately normal, 
justifying the use of 1-sigma error bars under the assumption of normality.

\begin{table}[h]
\centering
\caption{Quantitative evaluation results over 10 random seeds. We report each metric with the mean ± standard deviation (1$\sigma$). Except for 'PSNR' in super-resolution, all metrics passed the Shapiro-Wilk normality test ($p > 0.05$). We report the PSNR of super-resolution as the median $\pm$ interquartile range (IQR).}
\label{abl_stat}
\begin{adjustbox}{scale=0.9}
\begin{tabular}{cc|ccc}
\toprule
Category & Metric & Mean & 1-sigma Error Bar & p-value \\
\midrule
\multirow{2}{*}{Super-Resolution} &  PSNR  & 30.07 & $\pm$ 0.055    & 0.0425  \\
        &  LPIPS  & 0.0302 & $\pm$ 0.0002 & 0.6495   \\ \midrule
\multirow{2}{*}{3D Reconstruction} & PSNR      & 29.58 & $\pm$ 0.85     & 0.1319  \\
 & LPIPS     & 0.0382 & $\pm$ 0.0051  & 0.0911  \\ 
\bottomrule
\end{tabular}
\end{adjustbox}
\end{table}

\subsection{Non-GT MANO Parameters}
Although using ground-truth (GT) template parameters is a widely adopted strategy in 3D hand and body avatar reconstruction \cite{sHandAvatar, sHARP, sIm2Hands, sXhand, sOHTA, sEx}, and our method follows the same strategy, we additionally provide results where noise is added to the GT parameters. Tab. \ref{sup_non_gt} shows that MANO parameter errors do not have a critical effect on super-resolution performance, while they affect the quality of 3D hand reconstruction.

\begin{table}[h]
\centering
\caption{Quantitative results of showing the effectiveness of GT parameters.}
\label{sup_non_gt}
\begin{adjustbox}{scale=0.9}
\begin{tabular}{c|ccc|cc}
\toprule
\multirow{2}{*}{}   & \multicolumn{1}{c|}{\multirow{2}{*}{MPJPE (\textit{mm})}} & \multicolumn{2}{c}{Super-Resolution}            & \multicolumn{2}{|c}{3D Reconstruction} \\ \cmidrule(l){3-6} 
                    & \multicolumn{1}{c|}{}                            & PSNR & \multicolumn{1}{c|}{LPIPS} & PSNR              & LPIPS             \\ \cmidrule(l){2-6} 
Non-using GT Param. & 9.54                                             & 30.11      & 0.0306     & 27.18             & 0.0635            \\
Using GT Param.     & -                                                & 30.06      & 0.0302     & 29.88             &  0.0362            \\ \bottomrule

\end{tabular} 
\end{adjustbox}
\end{table}

\subsection{Additional Baseline Experiments}
We present additional experiments in Tab. \ref{sup:tab:add_exp} for HARP \cite{sHARP} and LiveHand \cite{sLiveHand}. HARP reconstructs a 3D hand using mesh subdivision with 3,093 vertices, which is not sufficient to represent a detailed hand geometric shape (significantly less than ours: 49,281 vertices). Also, assuming a one-point light condition differs from the benchmark settings used in our experiments, and yields geometric artifacts. LiveHand employs a low-resolution NeRF combined with a super-resolution network for real-time hand rendering. While efficient, LR NeRF and CNN-based SR module likely loses the 3D geometric information. Both methods encounter difficulties in reconstructing 3D hands from inconsistent super-resolved images and lack performance compared to ours.

\begin{table}[t]
\centering
\caption{Quantitative comparison of 3D reconstruction results. For fair comparison, our GIIF module was used for super-resolving images.}
\label{sup:tab:add_exp}
\begin{adjustbox}{scale=0.88}
\begin{tabular}{cccccc}
\toprule
SR Module & 3D Recon. Methods & PSNR & LPIPS & SSIM & P2P (mm) \\
\midrule
GIIF & HARP~\cite{sHARP}      & 26.25 & 0.0872 & 0.8773 & 5.20 \\
     & LiveHand~\cite{sLiveHand} & 26.91 & 0.0821 & 0.8805 & --   \\
     & XHand~\cite{sXhand}      & 27.71 & 0.0507 & 0.8876 & 3.43 \\
     & Ours                   & \textbf{29.88} & \textbf{0.0362} & \textbf{0.9206} & \textbf{2.16} \\
\bottomrule
\end{tabular}
\end{adjustbox}
\end{table}

\subsection{Arbitrary Scale Experiment}
\label{sec:arb}
Due to implicit-based image representation, our method can reconstruct a 3D hand with arbitrary resolution. We report the evaluation metrics in arbitrary upscaling factors along $\times$5.3, $\times$8, $\times$10.6, and $\times$16. Tab. \ref{sup_arb} and Fig. \ref{sup_fig_arb} shows the arbitrary scale super-resolution and 3D reconstruction results. We report PSNR and LPIPS metrics for each super-resolved image and 3D reconstructed hand. The results indicate that lowering the upscaling factor correspondingly increases the performance.

\begin{table}[h]
\centering
\caption{Quantitative results of arbitrary scale experiment. The two left columns show the PSNR and LPIPS results of super-resolved images and the right two columns present photometric metrics of a 3D reconstructed hand.}
\label{sup_arb}
\begin{adjustbox}{scale=0.9}
\begin{tabular}{@{}c|cc|cc@{}}
\toprule
             & \multicolumn{2}{c|}{Super-Resolution} & \multicolumn{2}{c}{3D Reconstruction} \\ \cmidrule(l){2-5} 
             & PSNR       & LPIPS      & PSNR              & LPIPS             \\ \midrule
$\times$32   & 28.82      & 0.0341     & 28.23             & 0.0409            \\ 
$\times$16   & 30.06      & 0.0302     & 29.88             & 0.0362            \\ 
$\times$10.6 & 30.52      & 0.0293     & 30.08             & 0.0343            \\
$\times$8    & 31.05      & 0.0262     & 30.23             & 0.0341            \\
$\times$5.3  & 31.42      & 0.0274     & 30.43             & 0.0334            \\ \bottomrule
\end{tabular}
\end{adjustbox}
\end{table}

\begin{figure*}[h]
  \centering
  \includegraphics[width=13.9cm]{fig/sup_arbitrary.pdf}
  \caption{Qualitative results of arbitrary upscaling factor experiment. Lowering the upscaling factor shows a more accurate and detailed representation of geometry and appearance.}
  \label{sup_fig_arb}
\end{figure*}

\subsection{Occlusion Ratio Experiment}
We also present complex occlusion experiments. Hand reconstruction is well-known to be challenging due to frequent self-occlusions and highly articulated poses. Our multi-view video setup is designed to alleviate these issues, yet detailed geometric reconstruction remains difficult in occluded regions. To simulate such challenging conditions, we reduce the number of training cameras to one or two and sample pose-varying frames. The occlusion rate is quantified through the percentage of invisible vertices of the hand in the camera viewing space. As expected, the reconstruction accuracy decreases as the occlusion rate increases, shown in the Tab. \ref{tab:occlusion}; however, not drastically.

\begin{table}[h]
\centering
\caption{Quantitative results under diverse occlusion rates. The occlusion rate is measured as the percentage of invisible vertices in the camera viewing space.}
\label{tab:occlusion}
\begin{adjustbox}{scale=0.9}    
\begin{tabular}{cccc}
\toprule
\textbf{Occlusion Rate (Train View \#)} & \textbf{PSNR} & \textbf{LPIPS} & \textbf{SSIM} \\
\midrule
24.7\% (1) & 25.54 & 0.0704 & 0.8636 \\
19.8\% (1) & 26.56 & 0.0597 & 0.8874 \\
9.43\% (2) & 28.05 & 0.0510 & 0.8986 \\
0\%        & 29.88 & 0.0362 & 0.9206 \\
\bottomrule
\end{tabular}
\end{adjustbox}
\end{table}

\subsection{Training and Inference Time}
We present the training and inference time specifications of SRHand. In the case of image super-resolution, GIIF processes each image in 3.5 ms, requiring a total of 17 seconds to upsample all training images. In contrast, a diffusion-based method \cite{sIDM} takes about 50 seconds per image, amounting to 5.5 hours in total. Tab. \ref{abl_spec} provides a detailed comparison of the training and inference times of our full model. SRHand achieves shorter training times and faster inference speeds, reaching up to 56 FPS, enabling real-time rendering.

\begin{table}[h]
\centering
\caption{Training and inference time comparison.}
\label{abl_spec}
\begin{adjustbox}{scale=0.9}
\begin{tabular}{@{}c|cc@{}}
\toprule
                  & Training Time (\textit{h}) & Inference Time (\textit{ms} / FPS) \\ \midrule
UHM \cite{sUHM}   & 5.5               & 139.5 / 7.2               \\ \midrule
SRHand            & \textbf{4.2}        & \textbf{17.8 / 56}        \\ \bottomrule
\end{tabular}
\end{adjustbox}
\end{table}

\section{More Qualitative Results}
\paragraph{GIIF.} First, we present additional qualitative results of GIIF compared with prior works in Fig. \ref{sup_liif}. Previous methods suffer from blurry textures and fail to represent geometric hand shapes accurately. Among prior methods, LIIF \cite{sLIIF} achieves the closest representation of the hand; however, it still struggles with blurry textures and unrealistic hand geometry, especially when fingers overlap. IDM \cite{sIDM} effectively captures hand-like texture appearances but produces hand geometry that deviates significantly from common hand shapes.

In both methods, incorporating a normal map as a condition improves the representation of hand geometry and textures. While both Geometric-aware LIIF and Geometric-aware IDM better capture hand structure and surface details, Geometric-aware LIIF still suffers from blurry textures and missing details, whereas Geometric-aware IDM exhibits noticeable differences from the referenced low-resolution image.

\paragraph{Geometric Enhancements.} We present more qualitative results of geometric enhancements in Fig. \ref{abl_ge}. We observe that our proposed method captures more details, such as nails and wrinkles, compared to XHand \cite{sXhand}.

\begin{figure}[h]
  \centering
  \includegraphics[width=8.9cm]{fig/sup_geometric_enhance.pdf}
  \caption{More qualitative results of showing geometric enhancements.}
  \label{abl_ge}
\end{figure}

\paragraph{SRHand.} We also present additional qualitative results of SRHand in Fig. \ref{sup_srhand}. Starting from low-resolution images, our method reconstructs realistic and high-fidelity 3D hands. Furthermore, by predicting the albedo color of the hand, our method enables relightable scenarios, unlike previous work \cite{sUHM}, which is relighted from the captured scene environment.

% Finally, we also present 512 $\times$ 512 size results, proving that our method is available on applications requiring detailed reconstructions. 

\section{Limitations and Future Works.}

\begin{figure}[h]
\centering
\includegraphics[width=12.cm]{fig/Generalization.pdf}
\caption{Qualitative results showing the generalization capability of our method to out-of-distribution scales, beyond the original dataset resolution.}
\label{sup:gen}
\end{figure}

We have demonstrated that SRHand performs well in the hand reconstruction domain, which is known for its high variance in pose articulations and view changes. All experiments are conducted on hand-focused datasets rather than a full-body captured dataset for fair comparison with prior works. Future work will be to extend our method to adapt to a full-body captured dataset. It remains to solve the occluded area caused by the body and to predict the accurate hand shape. 
Meanwhile, SRHand does demonstrate its generalization to out-of-distribution scales (see \textbf{Generalization Capability}). Our method can reconstruct high-fidelity 3D hands from 4K (4096$\times$4096) images, given sufficient GPU memory. Further applying SRHand to deformable objects and full-body human reconstruction remains a promising direction for future work, to capture more detailed and diverse 3D shapes.
% All experiments were conducted with the low-resolution images obtained by nearest-neighbor interpolation of the given HR images. 

% Note that most image super-resolution methods \cite{sLIIF, sIDM, sSRGNN, sINRv, sASR} are evaluated with LR-HR pairs obtained in the same manner, i.e. downsampling HR images. As some prior studies \cite{sRealESRGAN, sBSRGAN} have extended SR methods to real-world low-resolution images with complex real-world degradation simulation and common ringing and overshoot artifacts in the synthesis process, our method can also be extended to cover a wider range of degradation, which is our future work. 

\paragraph{Generalization Capability.}
We further demonstrate that our method enables hand reconstruction to out-of-distribution scales (\textit{e.g.} 512$\times$512) that far exceed the resolution of given images from the datasets as shown in Fig. \ref{sup:gen}. This supports practical deployment conditions, highlighting the robustness of our approach to unseen scales.

\paragraph{Social Impact.}
Hand geometry and motion patterns inherently contain biometric cues, which could pose potential privacy concerns. Our model is trained on the InterHand2.6M \cite{sInterHand2.6M} dataset, which was collected for public research purposes and does not include identity labels. The GIIF module is designed to learn a generalized hand prior conditioned on normal maps, rather than encoding identity-specific representations, and the 3D reconstruction pipeline does not capture personal identifiers in the absence of such information in the input images. This design substantially reduces direct privacy risks. Nevertheless, geometric characteristics such as finger proportions and hand shape may still implicitly serve as biometric signals. To mitigate these risks, our study employs only publicly available datasets, avoids training with identity annotations, and emphasizes identity-agnostic objectives in both the GIIF and reconstruction stages.

% artificially downsample the image from fixed resolution. 
% in synthetic environments, performing upscaling from low-resolution to limited resolution 256, 

% due to the ground-truth data existing problem. However, 
%compared to humans or objects. 
% , its evaluation has been limited to the hand domain, where textures are relatively uniform compared to clothed humans or other objects. Additionally, 

\begin{figure*}[]
  \centering
  \includegraphics[width=13.9cm]{fig/sup_LIIF_quali.pdf}
  \caption{More qualitative comparisons of GIIF and prior works. Zoom in to check the details.}
  \label{sup_liif}
\end{figure*}

\begin{figure*}[]
  \centering
  \includegraphics[width=13.7cm]{fig/sup_quali.pdf}
  \caption{More qualitative results of SRHand. Zoom in to check the details.}
  \label{sup_srhand}
\end{figure*}

\newpage
{
\small
~
%%%%%%%%%%%%%%%%%%%%%%%%%%%%%%%%%%%%%%%%%%%%%%%%%%%%%%%%%%%%
}

% \end{document}
